# Supplementary material for: Comparator automata in quantitative verification
Source: arXiv:1812.06569 source file (2022-07-28)
Supplement: Supplementary file 1 [file Appendix.tex]

\section{Limit Average Comparator}

\begin{lem}%
	\label{lem:sameAverage}
	Let $\Sigma = \{0, 1\dots \mu\}$. Let $L \in \Sigma^*$ s.t.\ the limit-average of all words in the language $L^{\omega}$ exists.
	Then average of all words in $L $ is the same.

	%Let $L$ be a regular language over finite words. Then $L^{\omega}$ will consist of words for which limit-average exists then the average of all words in $L$ is the same.
\end{lem}

\begin{proof}
	Suppose it is possible that two finite words $v_1$, $v_2\in L$ have different average. Let their length be $l_1$ and $l_2$ respectively with the average $a_1$ and $a_2$ respectively where $a_1 \neq a_2$.
	We will show the presence of a word $w \in L^{\omega}$ s.t.\ the limit-average of $w$ does not exist.

	Let $w_1 = v_1$. Then $\Av{w_1} = a_1$. Next, let $j_2$ be large enough to construct $w_2 = w_i v_2^{j_2}$ such that $\Av{w_2}\approx a_2$. Next, let $j_3$ be large enough to construct $w_3 = w_2 v_1^{j_3}$ such that $\Av{w_3} \approx a_1$.
	Continue constructing $w_4, w_5 \dots$ in a similar fashion s.t.\ their average change between  $a_2, a_1 \dots$ respectively.

	Let these $w = w_n$ as $n\rightarrow \infty$. Then $w \in L^{\omega}$, and since the average of its finite-length prefixes keeps changing between $a_1$ and $a_2$, limit-average of $w$ does not exist.

	This contradicts the premise that the limit-average of all words in $L^{\omega}$ exists. Therefore, our assumption that words $v_1$ and $v_2$ can have different average has been contradicted.

\end{proof}

\begin{lem}%
	\label{lem:sameLA}
	Let $\Sigma = \{0, 1, \dots \mu \}$. Let $L\subseteq \Sigma^*$ s.t.\ the average of all words in $\Sigma$ is the same, say $a$.
	Let $w \in L^{\omega}$ s.t.\ limit-average of  $w$ exists. Then $\LA{w} = a$
\end{lem}
\begin{proof}
Let $w = w_1w_2w_3\dots$. There exists infinitely many prefixes of $w$, prefix $w[i] = w_1w_2\dots w_i$ s.t. $\Av{w[i]} = a$.
Since we are given  that the limit-average of $w$ exists, it must be equal to $a$.
\end{proof}
